# Supplementary material for: Interactive Explainable Anomaly Detection for Industrial Settings
Source: arXiv:2410.12817 source file (2024-10-01)
Supplement: Supplementary file 1 [file appendix.tex]

\begin{figure}[h] 
    \includegraphics[width=0.9\linewidth]{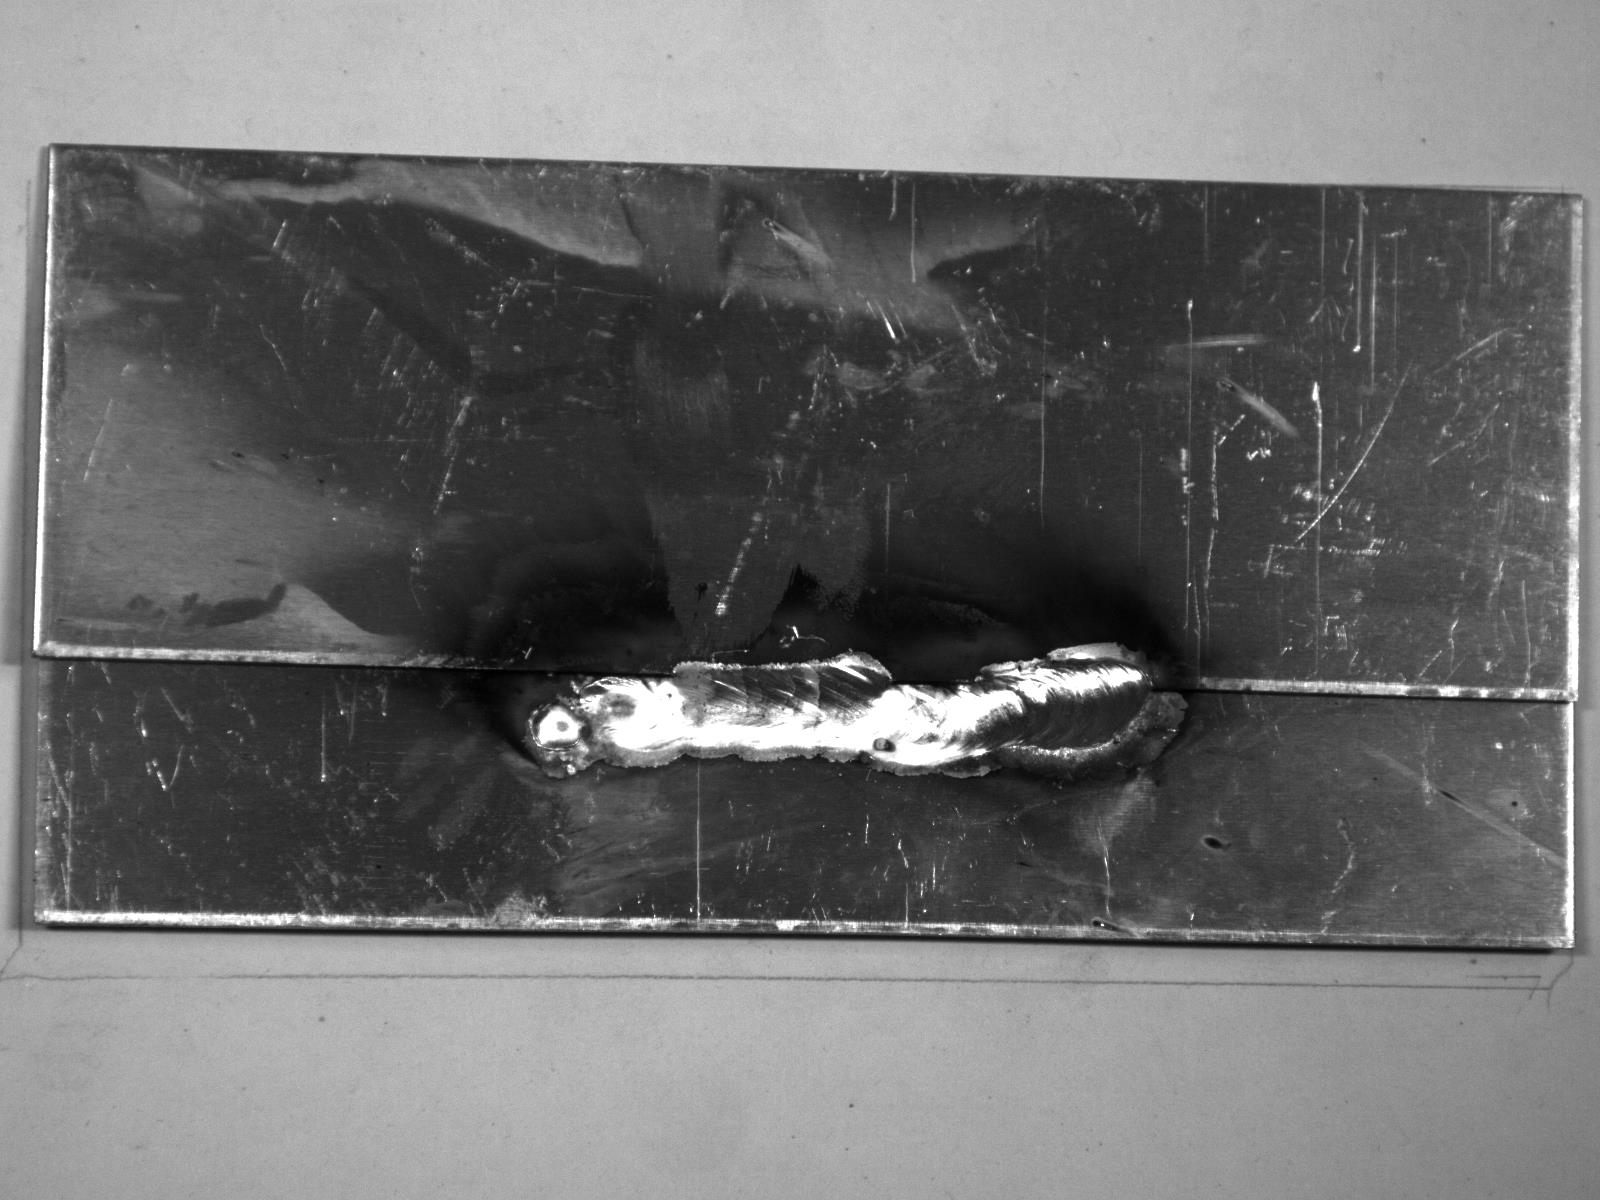}
    \caption{A welding seam with a burn through.} \label{burn_through} 
\end{figure}

\begin{figure}[h] 
    \includegraphics[width=0.9\linewidth]{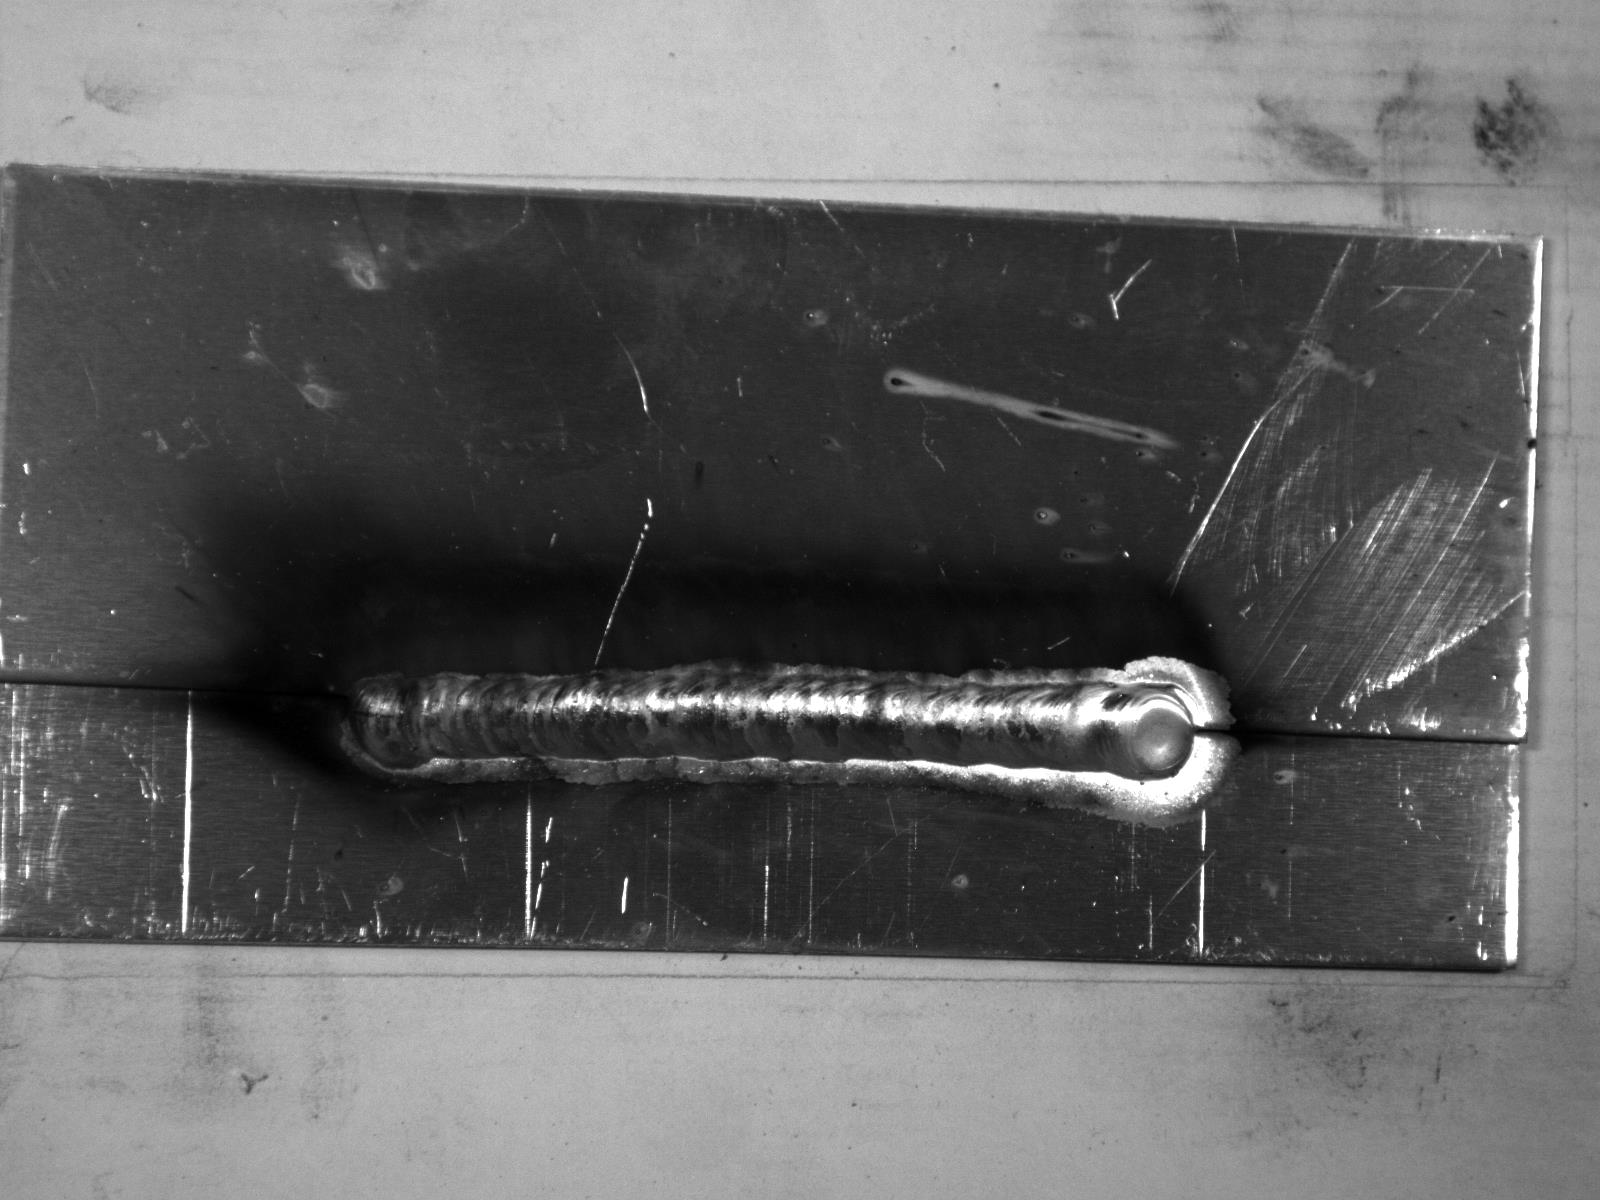}
    \caption{
    A black welding seam.} \label{black_seam} 
\end{figure}

\begin{figure}[h] 
    \includegraphics[width=0.9\linewidth]{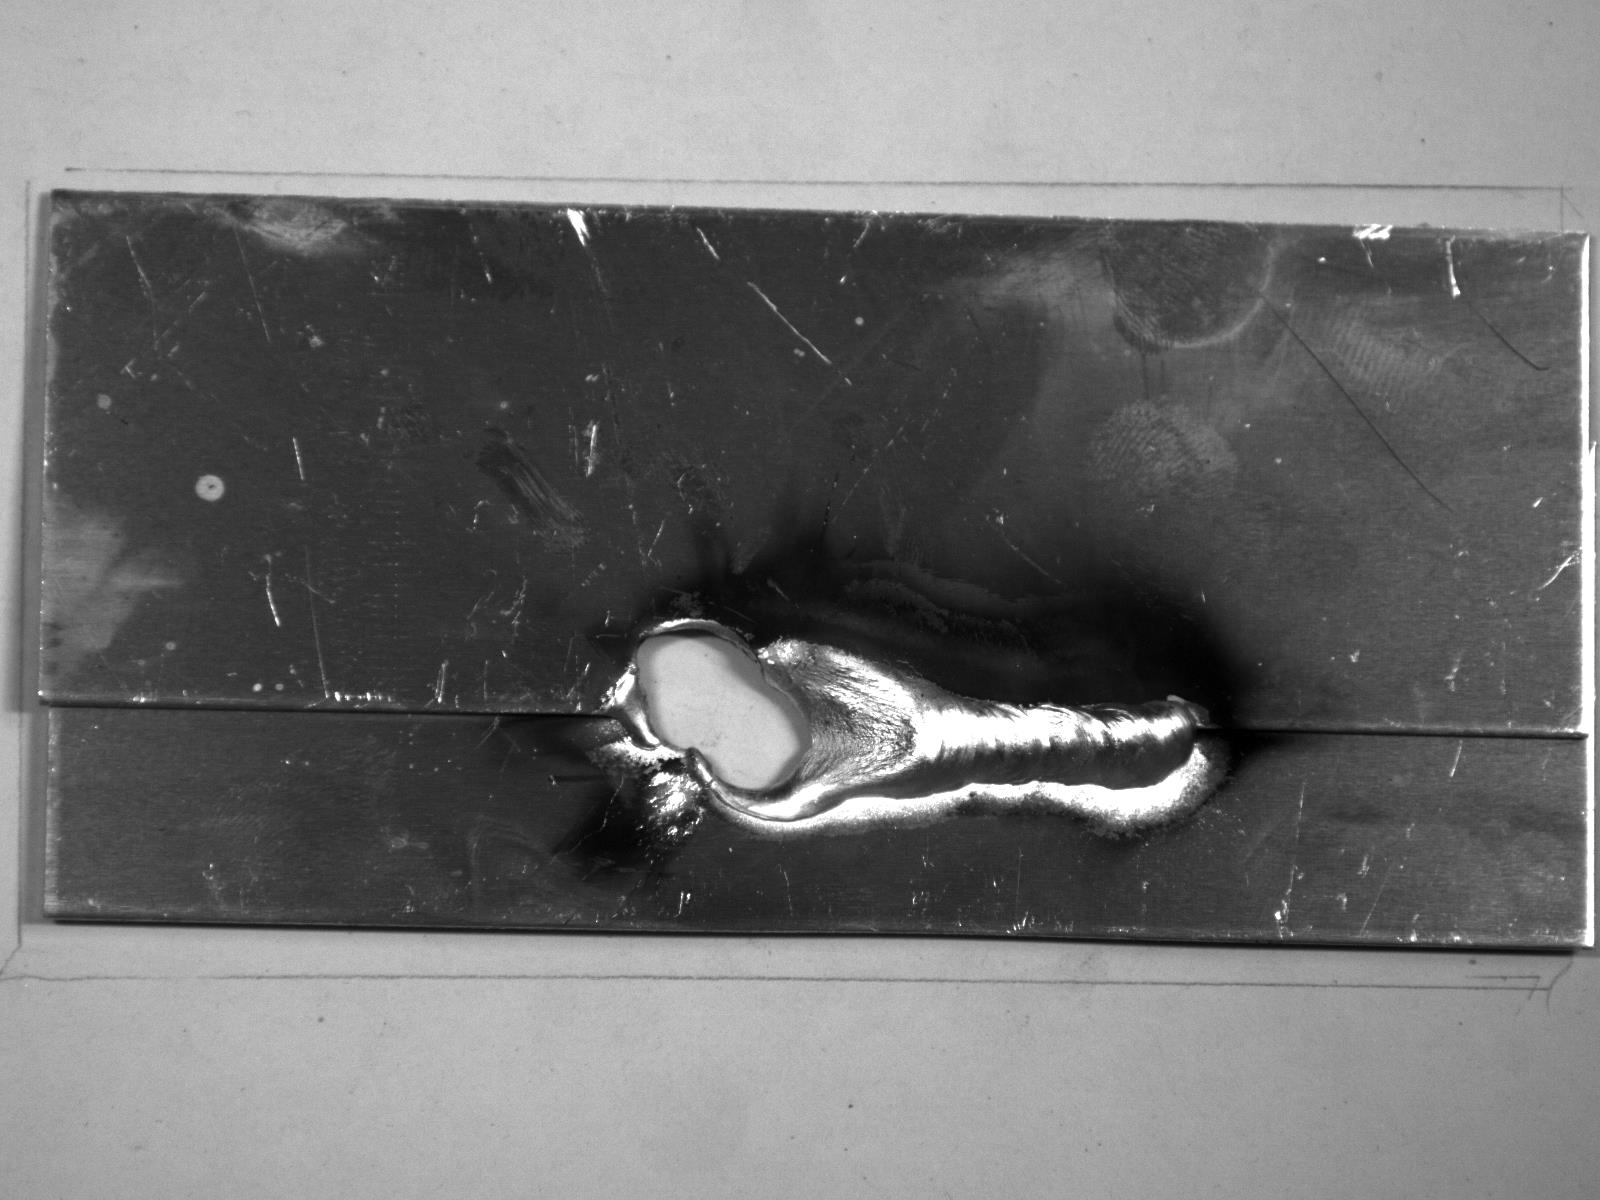}
    \caption{
    A welding seam with a hole in it.} \label{hole} 
\end{figure}

\begin{figure}[h] 
    \includegraphics[width=0.9\linewidth]{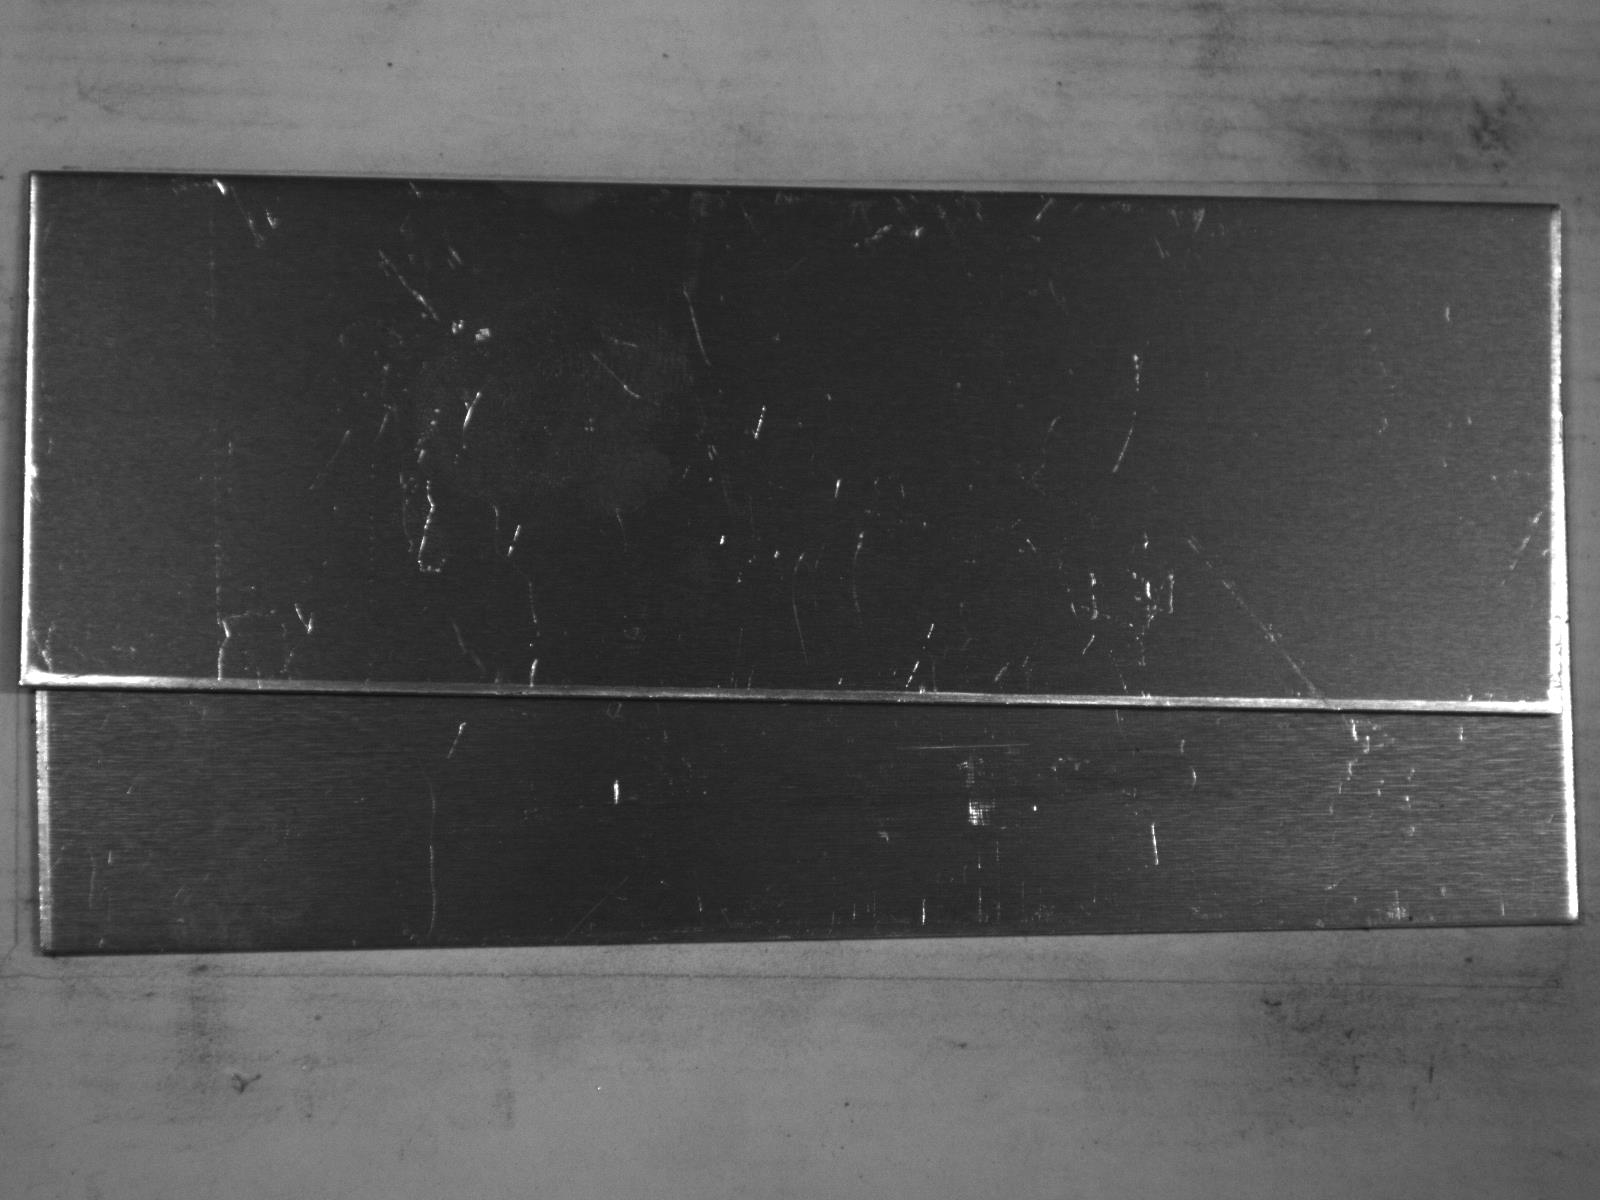}
    \caption{
    Plates with the welding seam missing.} \label{missing_seam} 
\end{figure}

\begin{figure}[h] 
    \includegraphics[width=0.9\linewidth]{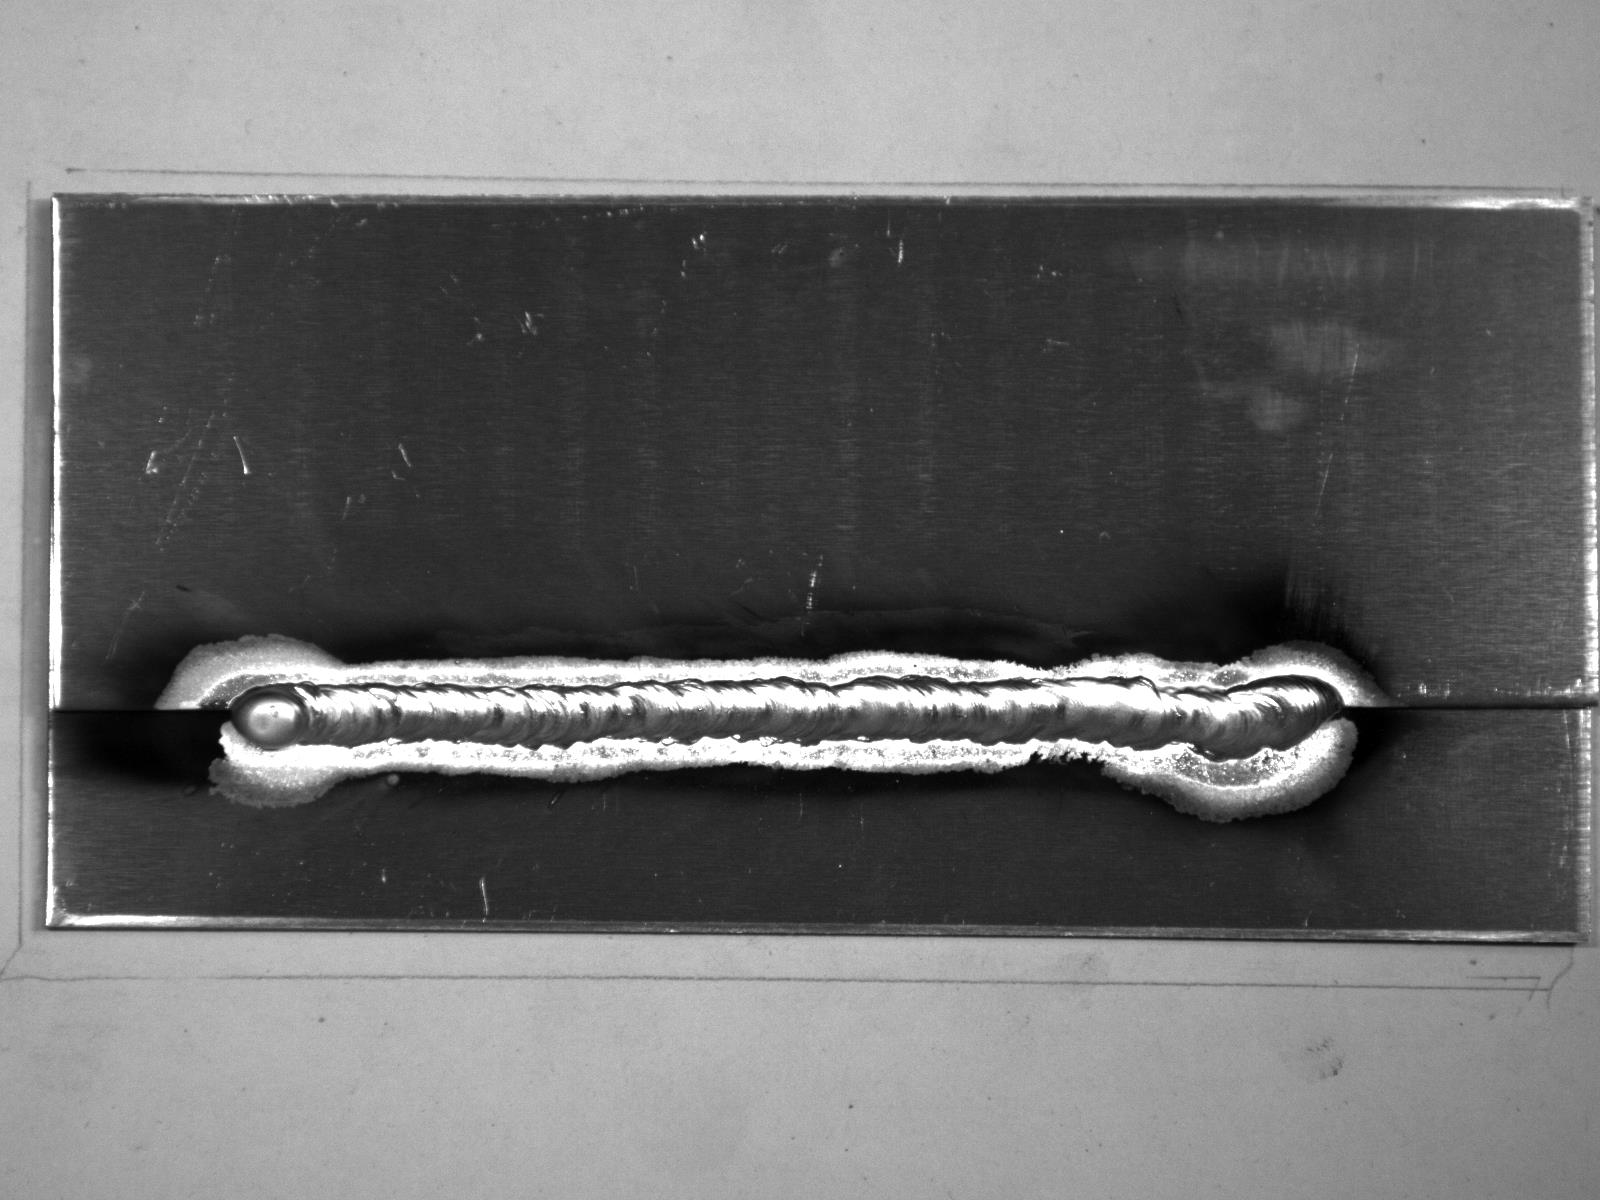}
    \caption{
    A welding seam with an irregular fish scale.} \label{irr_fish_scale} 
\end{figure}

\begin{figure}[h] 
    \includegraphics[width=0.9\linewidth]{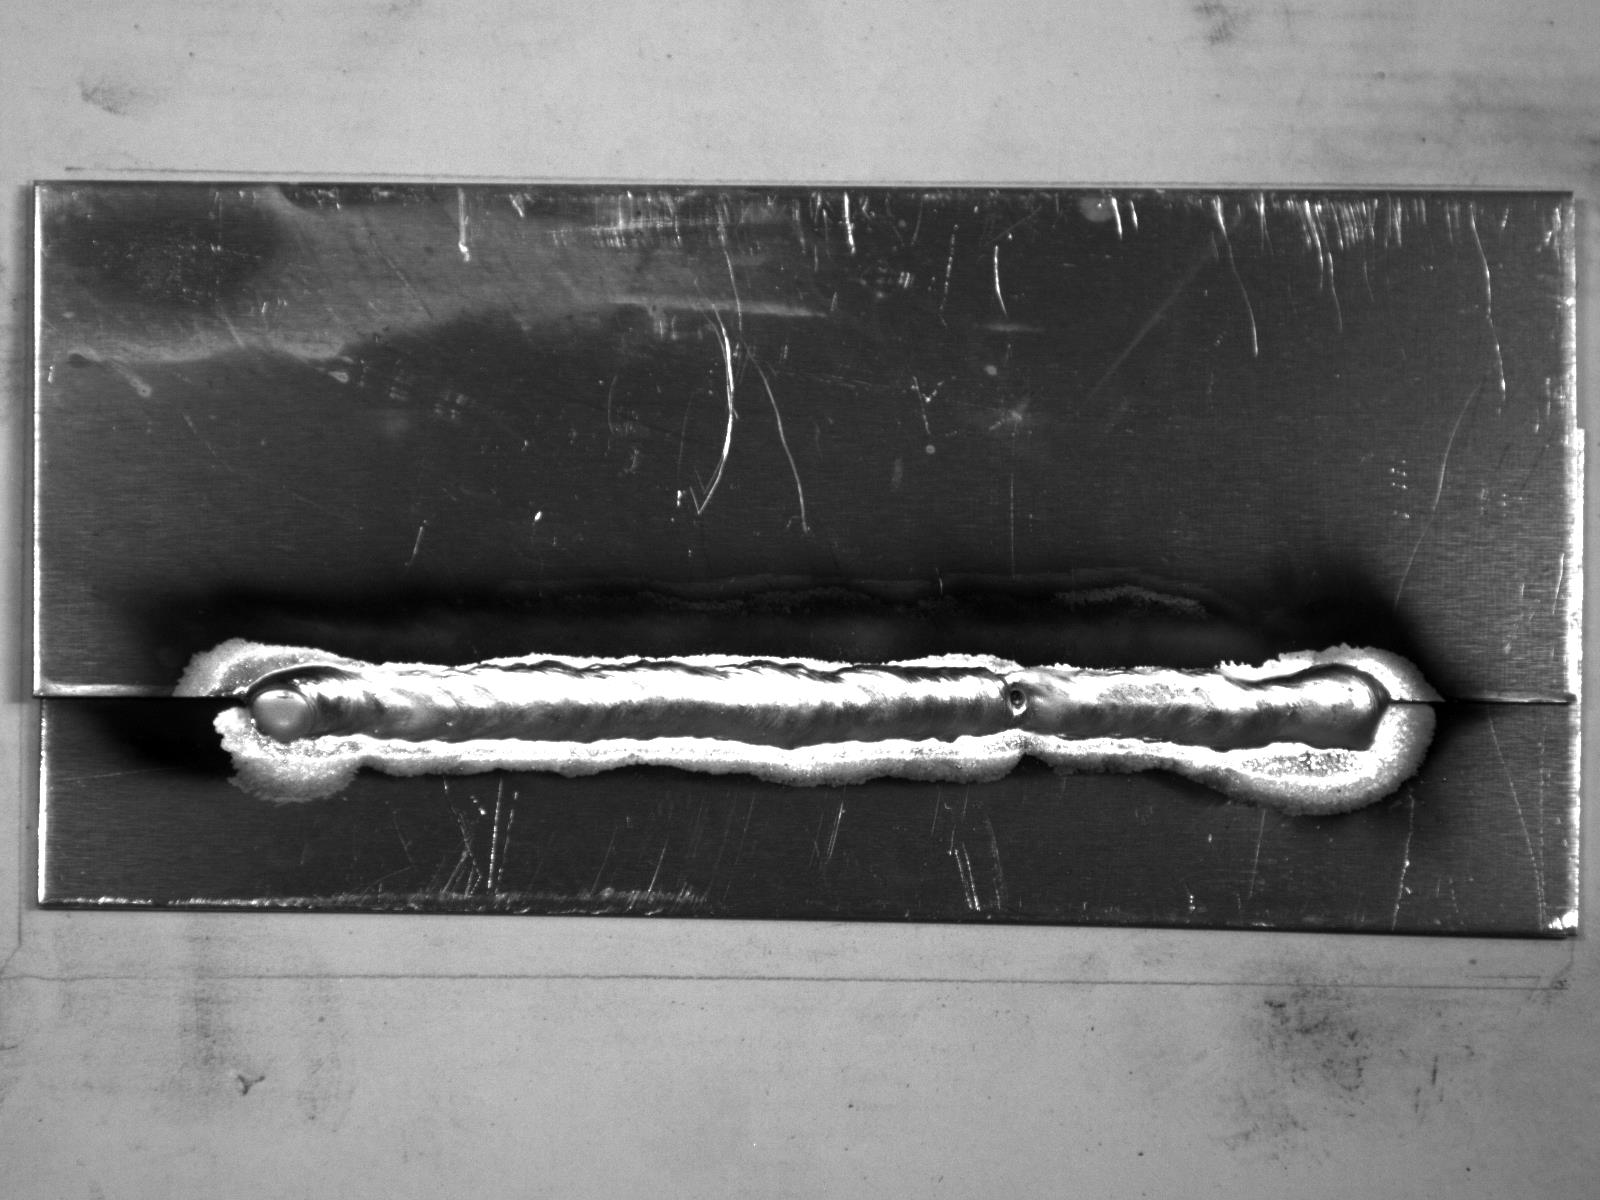}
    \caption{
    A welding seam containing a pore.} \label{pore} 
\end{figure}
